# Supplementary material for: Personalized Cross-Silo Federated Learning on Non-IID Data
Source: arXiv:2007.03797 source file (2021-12-14)
Supplement: Supplementary file 1 [file appendix.tex]

% !TEX root = ../main.tex

% ==============================================
% ===== Supplementary Material =================
% ==============================================
\nop{
\newpage
\appendix
\section{Algorithm}

\subsection{Problem Definition}

\begin{itemize}
    \item Define the non-IID federated learning problem.

    \item Emphasize the challenges of this problem.
\end{itemize}

\subsection{Attentive Multi-Task Learning (AMTL)}

\begin{itemize}
    \item Recall the \textbf{key ideas} to tackle the challenges.
    \begin{itemize}
        \item Let each client have its own model.
        \item Make similar models collaborate more (\textbf{non-linearity}).
    \end{itemize}
    
    \item Introduce the AMTL method in detail.
    \begin{itemize}
        \item Introduce the objective function and illustrate the intuition of why we would like to design it that way.
        \item Introduce our numerical solution and cite some papers to mention it's convergence.
        \item Introduce how to conduct our numerical solution in a \textbf{federated fashion} following the following steps of \textbf{Attentive Message Passing}
        \begin{itemize}
            \item Local updates on each client.
            \item Compute the attention strength between clients on the cloud.
            \item Aggregate client models using their attention strength in a message passing manner. (\textbf{be sure to highlight attention, message and message passing})
            \item A short summarization to explain why this preserves data privacy.
        \end{itemize}
        \item Summarize how the AMTL method can effectively tackle the convergence challenge and the customization challenge. (\textbf{This part should align well with our key ideas illustrated in the very beginning of this subsection.})
        \begin{itemize}
            \item How AMTL tackles the convergence challenge by letting each client have its own model.
            \item How AMTL tackles the customizatoin problem by making similar models collaborate more. (\textbf{Highlight the effect of $p$-norm in introducing non-linearity, cite Hinton's capsule net paper to imply the necessity of non-linearity in attention mechanism.})
            \item Prove that, for logistic regression/linear regression, the attention step is computing the canonical correlation between the data sets of different clients based on their models. Use this to \textbf{imply} the rationale of the attention mechanism, that is, the reason why we make similar models collaborate more is because \textbf{model similarity is highly related to data similarity.}
        \end{itemize}
    \end{itemize}
\end{itemize}

\subsection{Federated Attentive Message Passing (FedAMP))}

\begin{itemize}
    \item Illustrate why we want a heuristic to improve AMTL.
    \begin{itemize}
        \item Computing model similarity by inner product of model parameters is unstable, especially for large neural networks. Therefore, we use cosine similarity instead.
        \item $p$-norm is unstable in introducing non-linearity. Therefore, we follow Hinton's idea and use softmax to introduce non-linearity in attention mechanism.
    \end{itemize}
    
    \item Introduce the {FedAMP} algorithm in detail. (\textbf{This part should align well with the algorithmic structure of AMTL to give readers the feeling that we are only substituting some key components of the algorithmic framework of AMTL})
    
    \item Summarize that, we do not have convergence guarantee for {FedAMP}. But, it is simple and easy to implement and converges quite well in practice, even for deep neural networks. And it also achieves the best performance. (\textbf{Mention that attentive message passing can also lead to good clustering structure between data clients in an adaptive way without knowing the number of clusters before hand (cite the ``affinity propagation'' paper).})
\end{itemize}

\section{Problem Formulation}
Some notation:
\begin{itemize}
    \item $m$: number of clients;
    \item $n_i$: number of data samples on client $i$, where $i=1,2,\dots,m$;
    \item $d$: number of parameters in the neural network model;
    \item $w_i$: parameter of client $i$'s model, dimension is $d\times 1$.
    \item $W$: a matrix of size $d\times m$, whose $i$th column is $w_i$.
    \item $a_i$: attention vector for client $i$.
    \item $A$: attention matrix, whose $i$th column is $a_i$.
\end{itemize}
Our objective is
\begin{equation}
    \label{eq:main-obj}
    \begin{aligned}
    \min_{W,A} & \quad \sum_{i=1}^m \left(F_i(w_i) + \frac{\eta}{2}\|w_i\|_2^2\right) - \mbox{tr}(WAW^T) \\
    \mbox{s.t.} & \quad \|a_i\|_p \leq 1, \quad i=1,\dots,m, \\
    & \quad A \geq 0, \\
    & \quad \|W\|_F \leq R.
    \end{aligned}
\end{equation}
where $F_i$ is the empirical loss function of client $i$, i.e., 
\begin{equation}
    \label{eq:elm-i}
    F_i(w) = \frac{1}{n_i}\sum_{j=1}^{n_i} \ell(w_i;(x_j^i,y_j^i)),
\end{equation}
$p\in[1,2]$, and $\eta \geq \sqrt{m}$.

$w = (w_{i}| \forall i) \in \mathbb{R}^{n \times d}$, and the training samples $x =(x_{i}| \forall i) \in \mathbb{R}^{n \times r}$ with labels $y =(y_{i}| \forall i) \in \mathbb{R}^{n \times 1}$, the main objective function is:
\begin{equation}
    \min_{a, w} \sum_{i} F_i(w_i; (x_i, y_i)) - \sum_{i}\sum_{j \neq i} a_{ij}w_{i}^{\top}w_{j} + \eta \sum_{i}||w_{i}||_{2}^{2}
\end{equation}
s.t.
\begin{equation}
\label{equation_constraint-p-norm}
    ||a_{i}||_{p}^{p} \leq 1 \text{ and } a_{ij} \geq 0,  \quad \quad \forall i
\end{equation}

To solve the above problem, we can reformulate it as below:
\begin{equation}
    \min_{a, w} \sum_{i} F_i(w_i; (x_i, y_i)) - \sum_{i}\sum_{j \neq i} a_{ij}u_{i}^{\top}u_{j} + \eta \sum_{i}||w_{i}||_{2}^{2} \\
\end{equation}
s.t.
\begin{equation}
\label{equation_constraint-p-norm}
    u - w = 0, 
    ||a_{i}||_{p}^{p} \leq 1 \text{ and } a_{ij} \geq 0,  \quad \quad \forall i
\end{equation}
\textbf{}
Then we can apply penalty decomposition method to solve the above problem by solving a sequence of the following problem, 
\begin{equation}
    \min_{a, w, u} \sum_{i} F_i(w_i; (x_i, y_i)) - \sum_{i}\sum_{j \neq i} a_{ij}u_{i}^{\top}u_{j} + \eta \sum_{i}||u_{i}||_{2}^{2} + \frac{\rho}{2} \sum_{i} ||u_{i} - w_{i}||_{2}^{2}
\end{equation}
s.t.
\begin{equation}
\label{equation_constraint-p-norm}
    ||a_{i}||_{p}^{p} \leq 1 \text{ and } a_{ij} \geq 0,  \quad \quad \forall i
\end{equation}

Here, $a_{i} = (a_{ij}|\forall i \neq j) \in \mathbb{R}^{(n-1) \times 1}$, $u = (u_{i}| \forall i) \in \mathbb{R}^{n \times d}$, $F_i(w_i; (x_i, y_i))$ is the loss function for model indexed by $i$.

% By fixing $i$, the minimization of the objective function can be partitioned as $n$ separate minimization problems.
% \begin{equation}
% \sum_{i} \min_{a_{i}, w_{i}, u_{i}}(f_i(x) - \eta \sum_{j \neq i}a_{ij}u_{i}^{\top}u_{j} + \eta||w_{i}||_{2}^{2} + \frac{\rho}{2}||u_{i} - w_{i}||_{2}^{2})
% \end{equation}
% s.t. Eq (\ref{equation_constraint-p-norm}).

There are totally $3$ variables in the optimization objective function, by fixing the other $2$ variables, we divide the objective function as three subproblems to calculate the optimal value for each variable.

\textbf{Calculating the optimal $w$: (local update)}
\begin{equation}
    \min_{w} \sum_{i} (F_i(w_i; (x_i, y_i)) + \frac{\rho}{2}||u_i - w_i||_{2}^{2})
\end{equation}

\textbf{Calculating the optimal $a$: (attentive mechanism)}
\begin{equation}
    \min_{a} - \sum_{i} \sum_{j \neq i} a_{ij}u_{i}^{\top}u_{j}
    %\min_{a} \sum_{i} \sum_{j \neq i} a_{ij}e^{-u_{i}^{\top}u_{j}}
\end{equation}
s.t. Eq (\ref{equation_constraint-p-norm}).

\textbf{Calculating the optimal $u$: (message passing)}
\begin{equation}
    \min_{u} \sum_{i} (- \sum_{j \neq i} a_{ij}u_{i}^{\top}u_{j} + \eta ||u_{i}||_{2}^{2} + \frac{\rho}{2} ||u_i - w_i||_{2}^{2})
\end{equation}

\subsection{Comparison with Multi-Task Learning}
Some notation:
\begin{itemize}
    \item $m$: number of clients;
    \item $n_i$: number of data samples on client $i$, where $i=1,2,\dots,m$;
    \item $d$: number of parameters in the neural network model;
    \item $w_i$: parameter of client $i$'s model, dimension is $d\times 1$.
    \item $W$: a matrix of size $d\times m$, whose $i$th column is $w_i$.
    \item $\Omega$: a matrix of size $m\times m$, which induces cluster structures in $\{w_i\}_{i=1}^m$.
\end{itemize}
The classical formulation for multi-task learning is:
\begin{equation}
    \label{eq:MTL}
    \begin{aligned}
    \min_{W,\Omega} & \quad \underbrace{\sum_{i=1}^m\left(\frac{1}{n_i}\sum_{j=1}^{n_i} \ell(w_i;(x_j^i,y_j^i))\right)}_{\mbox{loss function}} + \underbrace{\alpha\eta(1+\eta)\cdot\mbox{tr}(W(\eta I + \Omega)^{-1}W^T)}_{\mbox{regularizer}} \\
    \mbox{s.t.} & \quad \mbox{tr}(\Omega) \leq k, \quad 0\preceq\Omega\preceq I
    \end{aligned}
\end{equation}
where $k$ is the number of clusters, $\eta = \beta/\alpha$,  $\beta$ is the regularization parameter for $\ell_2$ regularizers, i.e., $\|w_i\|_2^2$'s, and $\alpha$ is the regularization parameter for the regularizer that induces cluster structure among $w_i$'s. To allow distributed implementation, we employ the following reformulation of Eq.~(\ref{eq:MTL}):
\begin{equation}
    \label{eq:MTL-dist}
    \begin{aligned}
    \min_{W,U,\Omega} & \quad \sum_{i=1}^m\left(\frac{1}{n_i}\sum_{j=1}^{n_i} \ell(w_i;(x_j^i,y_j^i)) + \frac{\rho}{2}\|w_i - u_i\|_2^2\right) + \alpha\eta(1+\eta)\cdot\mbox{tr}(U(\eta I + \Omega)^{-1}U^T) \\
    \mbox{s.t.} & \quad \mbox{tr}(\Omega) \leq k, \quad 0\preceq\Omega\preceq I.
    \end{aligned}
\end{equation}

\medskip
\noindent
{\bf Numerical Solution:} (Consider the $k$th round)
\begin{itemize}
    \item[Step 1.] (client computation; update $w_i$'s) Every client $i$ receives $u_i^{k-1}$ from server. Then, every client $i$ performs local training with starting point  $u_i^{k-1}$ and proximal term $\frac{\rho}{2}\|w - u_i^{k-1}\|_2^2$, and find a new weight $w_i^k$, that is,
    \begin{equation}
    \label{eq:local-clients}
    w_i^k \approx \arg\min_w \frac{1}{n_i}\sum_{j=1}^{n_i}\ell(w; (x_j^i, y_j^i)) + \frac{\rho}{2}\|w - u_i^{k-1}\|_2^2.
    \end{equation}
    All clients send $\{w_i^k\}_{i=1}^m$ to server.
    \medskip
    
    \item[Step 2.] (server aggregation 1; update $\Omega$) The server find an $\Omega^k$ by letting
    \begin{equation}
        \label{eq:update-omega}
        \Omega^k = \arg\min_\Omega \left\{\mbox{tr}(U^{k-1}(\eta I + \Omega)^{-1}(U^{k-1})^T) : \ \mbox{tr}(\Omega) \leq k, \ 0\preceq\Omega\preceq I\right\}.
    \end{equation}
    To implement \eqref{eq:update-omega}, take the following four steps:
    \begin{itemize}
        \item[(i)] Compute $Z = (U^{k-1})^TU^{k-1}$
        \item[(ii)] Compute the eigenvalue decomposition of $Z$: 
        $$ Z = Q\Sigma Q^T, \quad  \mbox{where} \  \Sigma = \mbox{diag}(\sigma_1,\dots,\sigma_m). $$
        \item[(iii)] Solve the following convex optimization problem:
        \begin{equation}
            \label{eq:lambda-solve}
            (\lambda_1^*, \dots, \lambda_m^*) = \arg\min_{\lambda_1,\dots,\lambda_m} \left\{ \sum_{i=1}^m \frac{\sigma_i}{\eta + \lambda_i}: \ \sum_{i=1}^m \lambda_i = k, \ 0\leq \lambda_i \leq 1, \ \forall i\right\}.
        \end{equation}
        \item[(iv)] Set $\Omega^k = Q\Lambda Q^T$, where $Q$ is in (ii) and $\Lambda = \mbox{diag}(\lambda_1^*, \dots, \lambda_m^*)$ with $\lambda_i^*$'s in (iii).
    \end{itemize}
    \medskip
    
    \item[Step 3.] (server aggregation 2: update $u_i$'s) For every client $i$, the server find $U^k$ by
    \begin{equation}
        \label{eq:update-u}
        U^k = \arg\min_{U} \ \frac{\rho}{2}\|U - W^k\|_2^2 + \alpha\eta(1 + \eta)\cdot\mbox{tr}(U(\eta I + \Omega^k)^{-1} U^T).
    \end{equation}
    After simplification, one can verify that \eqref{eq:update-u} is equivalent with 
    \begin{equation}
        \label{eq:update-u-e}
        U^k = \frac{\rho}{2}W^k\left( \frac{\rho}{2}I + \alpha\eta(\eta+1)(\eta I + \Omega^k)^{-1}\right)^{-1}.
    \end{equation}
    To implement \eqref{eq:update-u-e}, we can use the $\Omega^k = Q\Lambda Q^T$ obtained in Step 2. Specifically, do the following steps:
    \begin{itemize}
        \item[(i)] Compute $\{\mu_i^*\}_{i=1}^m$ by
        $$ \mu_i^* = \frac{\rho}{2}\left( \frac{\rho}{2} + \frac{\alpha\eta(\eta+1)}{\eta+\lambda_i^*}\right)^{-1}, \quad i=1,2,\dots,m,$$
        where $\lambda_i^*$'s are computed in Step 2(iii).
        \item[(ii)] Set $M = Q\Sigma Q^T$, where $Q$ is in Step 2(ii) and $\Sigma = \mbox{diag}(\mu_1^*,\dots,\mu_m^*)$.
        \item[(iii)] Compute $U^k = W^kM$.
    \end{itemize}
\end{itemize}

\medskip
\noindent
{\bf Remark:} Step 1 and Step 2 can be performed simultaneously.

\medskip
\noindent
The question remaining is how to solve the $\lambda_i^*$'s in Step 2(iii). One can implement it via the following steps:
\begin{itemize}
    \item[(i)] Sort the $2m$ nonnegative real numbers: $\frac{\sigma_i}{\eta^2}$, $\frac{\sigma_i}{(\eta+1)^2}$, $i=1,2,\dots,m$. Denote them by 
    $$ 0 \leq a_{2m} \leq \dots \leq a_2 \leq a_1. $$
    For simplicity, we let $a_0 = +\infty$ and $a_{2m+1} = 0$.
    \item[(ii)] For $\ell=0$ to $2m$ do
        \begin{itemize}
            \item[(a)] Let $a_{\ell+1}<t<a_\ell$ be arbitrarily chosen. 
            \item[(b)] Find the following sets of indices:
            $$ \mathcal{I}_1=\left\{i:\frac{\sigma_i}{\eta^2}<t\right\}, \quad \mathcal{I}_2 = \left\{i:\frac{\sigma_i}{(\eta+1)^2}\leq t \leq \frac{\sigma_i}{\eta^2}\right\}, \quad \mathcal{I}_3 = \left\{i: \frac{\sigma_i}{(\eta+1)^2} > t\right\}. $$
            \item[(c)] Set 
            $$ t^* = \left(\frac{\sum_{i\in\mathcal{I}_2}\sqrt{\sigma_i}}{\eta|\mathcal{I}_2| - |\mathcal{I}_3| + k}\right)^2. $$
            \item[(d)] If $a_{\ell+1} \leq t^* \leq a_\ell$, then output the following $\lambda_i^*$'s and terminate:
            \begin{equation}
                \label{eq:lambda-star}
                \lambda_i^* = \left\{
                \begin{array}{cc}
                0, & \ i\in\mathcal{I}_1, \\
                \sqrt{\frac{\sigma_i}{t^*}} - \eta, & \ i\in\mathcal{I}_2, \\
                1, & \ i\in\mathcal{I}_3.
                \end{array}\right.
            \end{equation}
            Otherwise, continue the for loop.
        \end{itemize}
\end{itemize}

\subsection{Formulation 1}
We may also adopt the following formulation:
\begin{equation}
\label{eq:new-form}
\begin{aligned}
\min_{W\in\R^{d\times m}, \, A\in\R^{d\times d}} & \quad \sum_{i=1}^m F_i(w_i) + \frac{\lambda}{2}\sum_{i,j=1}^n \frac{\|w_i - w_j\|_2^2+\epsilon}{a_{ij}}, \\
\mbox{s.t.} \qquad & \quad \|a_j\|_p = 1, \quad j=1,2,\dots,m, \\
& \quad A \geq 0.
\end{aligned}
\end{equation}
Here, $a_{ij}$ is the $(i,j)$-th entry of $A$ and $a_j$ (resp.~$w_j$) is the $j$-th column of $A$ (resp.~$W$), and $p\geq 1$. To solve Problem \eqref{eq:new-form}, we introduce an auxiliary variable $U\in\R^{n\times d}$ and compute
\begin{equation}
\label{eq:new-form-U}
\begin{aligned}
\min_{W\in\R^{d\times m}, \, U\in\R^{d\times m}, \, A\in\R^{d\times d}} & \quad \sum_{i=1}^m F_i(w_i) + \frac{\lambda}{2}\sum_{i,j=1}^n \frac{\|u_i - u_j\|_2^2+\epsilon}{a_{ij}} + \frac{\rho}{2}\sum_{j=1}^m\|w_j - u_j\|_2^2, \\
\mbox{s.t.} \qquad & \quad \|a_j\|_p = 1, \quad j=1,2,\dots,m, \\
& \quad A \geq 0.
\end{aligned}
\end{equation}

\begin{algorithm}[t]
\DontPrintSemicolon
\SetKwInput{KwInput}{Input}               
\SetKwInput{KwOutput}{Output} 
\KwInput{$\lambda>0$, $\rho>0$, $\epsilon>0$, set $u_j^{(0)}=0$ for all $j$}
\KwOutput{the weight vectors ${w}_j$ and the latent vectors $u_j$ for all $j$}             
\For{$k=1,2,\dots$}{
Server sends the latent variables $u_i^{(k-1)}$ to each client \tcp*[f]{Broadcast}\\
Clients solve the following training problem for several epochs: \tcp*[f]{Local Training}
\begin{equation}
    \label{eq:update-W}
    w_i^{(k)} = \arg\min_w \, F_i(w) + \frac{\rho}{2}\|w - u_i^{(k-1)}\|_2^2.
\end{equation} 
\\
Clients send the updated $w_i^{(k)}$ back to Server \tcp*[f]{Collect}\\
Update the attentive matrix $A$. Specifically, for every column $j$, fist compute
$$ B^{(k)}_j = \left(\sum_{i=1}^m \left(\|u_i - u_j\|_2^2+\epsilon\right)^{\frac{p}{p+1}}\right)^{\frac{1}{p}}, $$
and then set every $a_{ij}$ as
\begin{equation}
    \label{eq:update-a}
    a_{ij} = \frac{\left(\|u_i - u_j\|_2^2+\epsilon\right)^{\frac{1}{p+1}}}{B^{(k)}_j}, \qquad i=1,\dots,m.
\end{equation}\\
Update the cloud vectors $u_i$'s \tcp*[f]{Aggregate}\\
First, form a matrix $C\in\mathbb{R}^{m\times m}$ such that
$$ c_{ij} = \left\{
\begin{aligned}
\sum_{\ell=1,\ell\neq i}^m (a_{\ell i})^{-1} + \sum_{\ell=1,\ell\neq i}^m (a_{i\ell})^{-1}     & \quad  \mbox{if} \ i=j, \\
-(a_{ij})^{-1} - (a_{ji})^{-1}     &  \quad \mbox{if} \ i\neq j.
\end{aligned}\right.
$$\\
Then, set 
\begin{equation}
    \label{eq:update-U-eq}
    U^{(k)} = \rho W^{(k)}(\lambda C + \rho I)^{-1}.
\end{equation}
Every column of $U^{(k)}$ is $u_i^{(k)}$.
}
\caption{{FedAMP} for Problem \eqref{eq:new-form-U}}
\label{alg:TSA}
\end{algorithm}

\section{Algorithm}
\textbf{Calculating the optimal $w$:} We use gradient descent to reach the optimal point for each $w_i$.
For simplicity, we define function $G_i(w_i)$ as:
\begin{equation}
    G_{i}(w_i) = F_i(w_i) + \frac{\rho}{2}||u_i - w_i||_{2}^{2}
\end{equation}
The derivative of the function $G_i(x)$ can be calculated by:
\begin{equation}
    \bigtriangledown G_i(w_i) = \bigtriangledown F_i(w_i; (x_i, y_i)) + \rho (w_i - u_i)
\end{equation}
$\bigtriangledown F_i(w_i; (x_i, y_i))$ is the gradient of the $w_i$ calculated by back propagation.
$w_i$ can be updated by:
\begin{equation}
\label{equation_train-wi}
    w_i = w_i - \lambda_{w} \bigtriangledown G_i(w_i)
\end{equation}
Here, $\lambda_{w}$ is the learning rate.

\textbf{Calculating the optimal $a$:} For each $a_i$, we solve the equivalent maximization problem as:
\begin{equation}
    \max_{a_{ij} \geq 0, \forall j} \quad t_{i}^{\top}a_{i}
\end{equation}
s.t.
\begin{equation}
\label{equation_constraint-p-norm_singlei}
    ||a_i|| _{p}^{p} \leq 1, a_{ij}\geq 0
\end{equation}
Here, $t_i = (t_{ij}|\forall i \neq j) \in \mathbb{R}^{(n-1) \times 1}$ and $t_{ij} = u_{i}^{\top}u_{j}$.

If $\forall j \neq i$, $t_{ij}=0$ satisfies, we set $a_{ij}=0$; otherwise, it has a dual problem formulation:
\begin{equation}
    \min_{\gamma}\max_{a_{ij} \geq 0, \forall j} \quad  t_{i}^{\top}a_{i} - \gamma (||a_{i}||_{p}^{p} - 1)
\end{equation}
s.t.
\begin{equation}
    t_{ij} - p\gamma \cdot (a_{ij})^{p-1} = 0, \quad \quad \forall j
\end{equation}

By fixing $\gamma$, we can calculate the optimal $a_{i}$ by:
\begin{equation}
    a_{ij} = (\frac{t_{ij}}{p\gamma})^{\frac{1}{p-1}}
\end{equation}

Substitute the above equation into the dual formulation, we formulate a new function $H(\gamma)$ with only one variable $\gamma$ as below:
\begin{equation}
    \min_{\gamma} H(\gamma) = \quad \gamma ^{\frac{1}{1-p}} [\sum_{j} t_{ij} \cdot (\frac{t_{ij}}{p})^{\frac{1}{p-1}} - \sum_{j} (\frac{t_{ij}}{p})^{\frac{p}{p-1}}] + \gamma
\end{equation}

For simplicity, we denote the invariable $k =  [\sum_{j} t_{ij} \cdot (\frac{t_{ij}}{p})^{\frac{1}{p-1}} - \sum_{j} (\frac{t_{ij}}{p})^{\frac{p}{p-1}}] = (p-1) \cdot p^{\frac{p}{1-p}} \cdot \sum_{j} t_{ij}^{\frac{p}{p-1}}$, and the derivative function is:
\begin{equation}
    \bigtriangledown H = \frac{k}{1-p} \gamma^{\frac{p}{1-p}} + 1
\end{equation}
When it equals $0$, we can achieve the optimal $\gamma$:
\begin{equation}
    \gamma = (\frac{p-1}{k})^{\frac{1-p}{p}}
\end{equation}
Thus $\forall j$, $a_{ij}$ can be calculated by:
\begin{equation}
\label{equation_update-ai}
\begin{split}
    a_{ij} & = [\frac{t_{ij}\cdot k^{\frac{1-p}{p}}}{p\cdot(p-1)^{\frac{1-p}{p}}}]^{\frac{1}{p-1}} \\
    & = \{\frac{t_{ij} \cdot [(p-1) \cdot p^{\frac{p}{1-p}} \cdot \sum_{j} t_{ij}^{\frac{p}{p-1}}]^{\frac{1-p}{p}}}{p\cdot(p-1)^{\frac{1-p}{p}}}\}^{\frac{1}{p-1}} \\
    & = [t_{ij} \cdot (\sum_{j} t_{ij}^{\frac{p}{p-1}})^{\frac{1-p}{p}}]^{\frac{1}{p-1}} \\
    & = {t_{ij}}^{\frac{1}{p-1}} \cdot (\sum_{j} t_{ij}^{\frac{p}{p-1}})^{-\frac{1}{p}}
\end{split}
\end{equation}

\textbf{Calculating the optimal $u$:} For each $u_i$, we define function $Q_i(u_i)$ as:
\begin{equation}
    Q_i(u_i) = - \sum_{j \neq i} a_{ij}u_{i}^{\top}u_{j} + \eta ||u_{i}||_{2}^{2} + \frac{\rho}{2} ||u_i - w_i||_{2}^{2}
\end{equation}
The derivative of $Q_i(u_i)$ is:
\begin{equation}
    \bigtriangledown Q_i(u_i) = - \sum_{j \neq i} a_{ij}u_j + 2\eta u_{i} + \rho (u_i - w_i)
\end{equation}
When the derivative equals $0$, the optimal $u_i$ can be calculated by the following equation:
\begin{equation}
\label{equation_update-ui}
    u_i =  \frac{(\sum_{j \neq i} a_{ij}u_j) + \rho w_i}{2\eta + \rho} 
\end{equation}

{\bf Calculating the optimal $u$:} When update $U$, consider the problem
\begin{equation}
    \label{eq:update-U-new}
    U^+ = \arg\min_U \sum_{i=1}^m\left(\frac{\rho}{2}\|u_i - w_i\|_2^2 + \eta\|u_i\|_2^2\right) - \sum_{i=1}^m\sum_{j\neq i} a_{ij}u_i^Tu_j
\end{equation}
Let $A$ be the matrix with $a_{ij}$ and $a_{ii} = 0$ for all $i$. Then,
$$ 
\begin{aligned}
\sum_{i=1}^m\sum_{j\neq i} a_{ij}u_i^Tu_j & = \langle A, U^TU\rangle = \mbox{tr}(A^TU^TU) = \mbox{tr}(UA^TU^T) \\
\sum_{i=1}^m\left(\frac{\rho}{2}\|u_i - w_i\|_2^2 + \eta\|u_i\|_2^2\right) & = \frac{\rho}{2}\|U - W\|_F^2 + \eta\|U\|_F^2 = \frac{\rho}{2}\|U - W\|_F^2 + \eta\mbox{tr}(UU^T).
\end{aligned}
$$
\textcolor{red}{
Thus, \eqref{eq:update-U-new} can be written as
\begin{equation}
\label{eq:update-U-opt}
U^+ = \arg\min_U \frac{\rho}{2}\|U - W\|_F^2 + \mbox{tr}(U(\eta I - A^T)U^T). 
\end{equation} 
Since \eqref{eq:update-U-opt} is a quadratic minimization, its solution is bounded if and only if it is convex. By taking its Hessian, we have
$$ \rho I + 2\eta I - A - A^T \succeq \mathbf{0}. $$
Hence, we need 
$$ \frac{\rho}{2} + \eta \geq \|A\|_2, $$
where $\|\cdot\|_2$ is the operator norm, i.e., largest singular value. Because $A$ has $m$ columns, with each column being $a_j$, we have
$$ \|A\|_2 \leq \sqrt{m}\sum_{j=1}^m\|a_j\|_2, $$
where $\|a_j\|_2$ is the vector 2-norm. For $p\in[1,2]$, we have $\|a_j\|_2 \leq \|a_j\|_p \leq 1$, which yields
$$ \|A\|_2 \leq \sqrt{m} $$ 
for any possible $A$ satisfying our requirement. This is why we need to set 
$$ \frac{\rho}{2} + \eta \geq \sqrt{m}. $$
}
Taking derivative, we obtain
$$ \mathbf{0} = \rho(U^+ - W) + U^+(2\eta I - A - A^T). $$
Thus,
$$ U^+ = \rho W\left((\rho+2\eta )I - A - A^T\right)^{-1}. $$

\begin{algorithm}[!t]
\caption{An algorithm}
\KwData{The training data set $x$,
the maximum iteration limitation $iter_{max}$ and the maximum epoch limitation $epoch_{max}$}
\KwResult{$w$, $a$, $u$}
\textbf{Initialization:}\\
\For{$i$ from $1$ to $n$}{
    Pre-train $w_i$ by its own data\;
    Set $u_i := w_i$\; 
}
\For{$i$ from $1$ to $n$}{
Update $a_i$ by Eq (\ref{equation_update-ai})\;
}
\For{$i$ from $1$ to $n$}{
Update $u_i$ by Eq (\ref{equation_update-ui})\;
}

\textbf{Training:}\\
\While{$iter$ from $1$ to $iter_{max}$}{
\For{$i$ from $1$ to $n$}{
    \For{$epoch$ from $1$ to $epoch_{max}$}{
        Training $w_i$ by Eq (\ref{equation_train-wi})\;
    }
}

\For{$i$ from $1$ to $n$}{
Update $a_i$ by Eq (\ref{equation_update-ai})\;
}
\For{$i$ from $1$ to $n$}{
Update $u_i$ by Eq (\ref{equation_update-ui})\;
}
}
\end{algorithm}

\section{Experiments}

For each data set, we have three types of distribution settings: IID, pathological Non-IID, and \textit{practical} Non-IID. The IID setting is data distributed uniformly random across different clients, and the pathological Non-IID setting follows the steps used by \cite{mcmahan2016communication}, where they partitioned the data set based on labels and for each client draw samples from two classes. The \textit{practical} Non-IID settings are specified as follows. 

\textbf{Baselines}
\begin{itemize}
    \item Centralized
    \item Separated
    \item FedAvg
    \item FedProx
    \item MOCHA 
\end{itemize}

\subsection{Parameter Analysis}
Analyze the influence of parameters in our methods.

\subsection{Effect of Data Distribution}
\begin{itemize}
    \item Evaluate the performance of all baseline methods under three different data distribution settings.
    \item Analyze the influence of data distributions on the performance of all compared methods. (Attack the weakness of baseline methods, and claim our advantage.)
    \item Demonstrate the good performance of both {FedAMP} and {HeurFedAMP}.
    \item Summarize that our methods achieve these good results by attentive message passing.
\end{itemize}

\subsection{Communication Efficiency}
Illustrate that for federated learning, the bottle neck of efficiency is communication with cloud for aggregation. This motivates our experiment to evaluate convergence speed with respect to the number of cloud aggregations. (\textbf{It's the best if we could cite some paper with similar experiment settings})
\begin{itemize}
    \item Evaluate the speed of convergence with respect to the number of aggregations on the cloud. (FedAvg and FedProx can still converge if they frequently conduct aggregations. But, this operation is time consuming due to the latency of communication)
    \item Demonstrate the advantage of our method in using a very small number of aggregations to converge fast.
\end{itemize}

\subsection{Robustness Against Dropped Clients}
Demonstrate our method achieves a comparable performance facing dropped clients.

\huang{Tables:}
\begin{table}[h!]
\centering
\begin{tabular}{ |c|c c c| } 
 \hline
 Baselines & IID & Non-IID Non-grouping & Non-IID Grouping \\ 
 \hline
 FedAMP &  &  &  \\ 
 Heuristic &  &  & \\ 
 Centralized &  &  & \\
 Separate &  &  & \\
 FedAvg &  &  & \\
 FedProx &  &  & \\
 FedAvg\_finetune &  &  & \\
 FedProx\_finetune &  &  & \\
 MOCHA &  &  & \\
 \hline
\end{tabular}
\caption{MNIST}
\end{table}

\begin{table}[h!]
\centering
\begin{tabular}{ |c|c c c| } 
 \hline
 Baselines & IID & Non-IID Non-grouping & Non-IID Grouping \\ 
 \hline
 FedAMP &  &  &  \\ 
 Heuristic &  &  & \\ 
 Centralized &  &  & \\
 Separate &  &  & \\
 FedAvg &  &  & \\
 FedProx &  &  & \\
 FedAvg\_finetune &  &  & \\
 FedProx\_finetune &  &  & \\
 MOCHA &  &  & \\
 \hline
\end{tabular}
\caption{Fashion-MNIST}
\end{table}

\begin{table}[h!]
\centering
\begin{tabular}{ |c|c c c| } 
 \hline
 Baselines & IID & Non-IID Non-grouping & Non-IID Grouping \\ 
 \hline
 FedAMP &  &  &  \\ 
 Heuristic &  &  & \\ 
 Centralized &  &  & \\
 Separate &  &  & \\
 FedAvg &  &  & \\
 FedProx &  &  & \\
 FedAvg\_finetune &  &  & \\
 FedProx\_finetune &  &  & \\
 MOCHA &  &  & \\
 \hline
\end{tabular}
\caption{Extended-MNIST}
\end{table}

\begin{table}[h!]
\centering
\begin{tabular}{ |c|c c c| } 
 \hline
 Baselines & IID & Non-IID Non-grouping & Non-IID Grouping \\ 
 \hline
 FedAMP &  &  &  \\ 
 Heuristic &  &  & \\ 
 Centralized &  &  & \\
 Separate &  &  & \\
 FedAvg &  &  & \\
 FedProx &  &  & \\
 FedAvg\_finetune &  &  & \\
 FedProx\_finetune &  &  & \\
 MOCHA &  &  & \\
 \hline
\end{tabular}
\caption{CIFAR-10}
\end{table}
}

% ==============================================
% ===== Supplementary Material =================
% ==============================================
\clearpage
\appendix
\begin{center}
{\Large \bf Appendix}
\end{center}
%\par\noindent\rule{\textwidth}{1pt}
\setcounter{section}{0}
In this appendix, we provide the proofs for Theorem 1 and 2 in Sections~\ref{sec:analysis-convex} and \ref{sec:analysis-ncvx}, respectively. In addition, we show more extensive experimental results in Section \ref{sec:supexp}.

\section{Proof of Theorem \ref{thm:analysis-convex}}\label{sec:analysis-convex}
The proof of Theorem \ref{thm:analysis-convex} is an adaptation of the proof in \cite{bertsekas2011incremental} to our setting.
Throughout the proof, we denote by $\mG^*$ the optimal value and $W^*$ an optimal solution of problem \eqref{eq:our-form}. Recall that {FedAMP} follows the update formula \eqref{eq:grad-descent-intro} and \eqref{eq:ppa-intro}. 
% Recall that if $\beta_k = \alpha_k/\lambda$ for all $k$, {FedAMP} follows the update formula \eqref{eq:grad-descent-intro} and \eqref{eq:ppa-intro}. 
Since $\mF$ is convex, the objective function in \eqref{eq:ppa-intro} is strongly convex with modulus $\lambda/\alpha_k$. This, together with the fact that $W^k$ is the optimal solution of \eqref{eq:ppa-intro}, implies that
$$ 
\begin{aligned} 
& \mF(W^k) + \frac{\lambda}{2\alpha_k}\|W^k - U^k\|^2 \\
& \leq \mF(W^*) + \frac{\lambda}{2\alpha_k}\|W^* - U^k\|^2 - \frac{\lambda}{2\alpha_k}\|W^* - W^k\|^2. 
\end{aligned}
$$
Upon rearrangement, we obtain
\begin{equation}
\label{eq:decrease-ppa}
\|W^k - W^*\|^2 + \frac{2\alpha_k}{\lambda}(\mF(W^k) - \mF(W^*)) \leq \|U^k - W^*\|^2.
\end{equation}
Since $U^k$ is generated by \eqref{eq:grad-descent-intro}, we have
\begin{align*}
& \|U^k - W^*\|^2 = \|W^{k-1} - \alpha_k\nabla\mA(W^{k-1}) - W^*\|^2 \\
& = \|W^{k-1} - W^*\|^2 - 2\alpha_k\langle\nabla \mA(W^{k-1}), W^{k-1} - W^*\rangle \\ 
& \quad + \alpha_k^2 \|\nabla\mA(W^{k-1})\|^2.
\end{align*}
Besides, since $\mA$ is convex, one has
$$ \mA(W^*) \geq \mA(W^{k-1}) + \langle \nabla \mA(W^{k-1}), W^* - W^{k-1}\rangle $$
By combining the above two inequalities and using Assumption \ref{ass:bound}, we obtain
\begin{equation}
    \label{eq:decrease-gd}
    \begin{aligned}
    & \|U^k - W^*\|^2 + 2\alpha_k(\mA(W^{k-1}) - \mA(W^*)) \\ & \leq \|W^{k-1} - W^*\|^2 + \frac{\alpha_k^2B^2}{\lambda^2}
    \end{aligned}
\end{equation}
Adding up \eqref{eq:decrease-gd} and \eqref{eq:decrease-ppa} and using the definition $\mG = \mF + \lambda\mA$ yield 
\begin{equation}
    \label{eq:recursion}
    \begin{aligned}
    & \|W^k - W^*\|^2 + \frac{2\alpha_k}{\lambda}\left(\mF(W^k) + \lambda\mA(W^{k-1}) - \mG^*\right) \\ & \leq \|W^{k-1} - W^*\|^2  + \frac{\alpha_k^2B^2}{\lambda^2}.
    \end{aligned}
\end{equation}
Moreover, by the convexity of $\mF$ and Assumption \ref{ass:bound}, we have, with any $Y\in\partial \mF(W^{k-1})$, that 
$$ 
\begin{aligned}
& \mF(W^k) - \mF(W^{k-1}) \geq \langle Y, W^k - W^{k-1}\rangle \\
& \geq -\|Y\|\|W^k - W^{k-1}\| \geq -B\|W^k - W^{k-1}\|.
\end{aligned}
$$
Also, it follows from the optimality condition of \eqref{eq:ppa-intro} that
$$ 0 = \tilde{\nabla} \mF(W^k) + \frac{\lambda}{\alpha_k}(W^k - U^k) $$
for some $\tilde{\nabla}\mF(W^k)\in\partial \mF(W^k)$, which, together with \eqref{eq:grad-descent-intro} and Assumption \ref{ass:bound}, yields 
$$ 
\begin{aligned}
& \|W^k - W^{k-1}\| = \left\| U^k - \frac{\alpha_k}{\lambda}\tilde{\nabla}\mF(W^k) - W^{k-1}\right\| \\
& = \left\|\alpha_k\nabla\mA(W^{k-1}) + \frac{\alpha_k}{\lambda}\tilde{\nabla}\mF(W^k)\right\| \leq \frac{2\alpha_kB}{\lambda}. 
\end{aligned}
$$
Upon combining the above two inequalities, we obtain
$$ \mF(W^k) \geq \mF(W^{k-1}) - \frac{2\alpha_kB^2}{\lambda}. $$
Substituting this into \eqref{eq:recursion} and using the definition $\mG = \mF + \lambda\mA$ yield
\begin{align*}
& \|W^k - W^*\|^2 \\
& \leq \|W^{k-1} - W^*\|^2 - \frac{2\alpha_k}{\lambda}\left(\mG(W^{k-1}) - \mG^*\right) + \frac{5\alpha_k^2B^2}{\lambda^2},
\end{align*}
which, after rearrangement, leads to
\begin{equation}\label{eq:convex-recur}
\begin{aligned}
& \mG(W^{k-1}) - \mG^* \\
& \leq \frac{\lambda}{2\alpha_k}\|W^{k-1} - W^*\|^2 - \frac{\lambda}{2\alpha_k}\|W^k - W^*\|^2 + \frac{5\alpha_kB^2}{2\lambda}. 
\end{aligned}
\end{equation}
We now consider the case where $\alpha_k = \alpha = \lambda/\sqrt{K}$ for all $k=1,2,\dots,K$. Then, by summing up \eqref{eq:convex-recur} from $k=1$ to $k=K$, we obtain
$$ 
\begin{aligned}
& K\cdot \left(\min_{0\leq k\leq K-1} \mG(W^k) - \mG^*\right) \\
& \leq \sum_{k=0}^{K-1} \mG(W^k) - \mG^* \leq \frac{\lambda}{2\alpha}\|W^0 - W^*\|^2 + \frac{5K\alpha B^2}{2\lambda}. 
\end{aligned}
$$
Upon dividing both sides of the above inequality by $K$ and using $\alpha = \lambda/\sqrt{K}$, we obtain the first desired result in Theorem~\ref{thm:analysis-convex}. Besides, upon multiplying both sides of \eqref{eq:convex-recur} by $\alpha_k$ and summing it up from $k=1$, one has
$$ \sum_{k=1}^\infty \alpha_k\left(\mG(W^{k-1}) - \mG^*\right) \leq \frac{\lambda}{2}\|W^0 - W^*\|^2 + \frac{5B^2}{2\lambda}\sum_{k=1}^\infty\alpha_k^2. $$
Then, for the case where $\alpha_k$ satisfies $\sum_{k=1}^\infty\alpha_k = \infty$ and $\sum_{k=1}^\infty\alpha_k^2 < \infty$, we obtain
$$ \sum_{k=1}^\infty \alpha_k\left(\mG(W^{k-1}) - \mG^*\right) < \infty, $$
which, together with $\sum_{k=1}^\infty\alpha_k = \infty$ and $\alpha_k>0$ for all $k$, yields the second desired result in Theorem \ref{thm:analysis-convex}.

% This, together with \eqref{eq:recursion}, leads to
% \begin{equation}
%     \label{eq:recursion-all}
%     \begin{aligned}
%     \|W^k - W\|^2 & \leq \|W^{k-1} - W\|^2 - \frac{2\alpha_k}{\lambda}\left(\mF(W^k) + \lambda\mA(W^{k-1}) - \mG(W)\right) + \frac{\alpha_k^2B^2}{\lambda},
%     \end{aligned}
% \end{equation}

\section{Proof of Theorem \ref{thm:analysis-ncvx}}\label{sec:analysis-ncvx}
The proof of Theorem \ref{thm:analysis-ncvx} is motivated by the analysis in \cite{li2019incremental}. Define the function $\hat{\mG}:\R^d\rightarrow\R$ as
\begin{equation}
    \label{eq:envelope-func}
    \hat{\mG}(W) = \min_{V\in\R^{d\times m}} \mG(V) + 2L\|V - W\|^2,
\end{equation}
where $L$ is the Lipschitz constant of $\nabla \mA$. Also, given any $W\in\R^{d\times m}$, we denote by $\bar{W}$ an optimal solution of the minimization problem in \eqref{eq:envelope-func}, {\it i.e.}, $ \hat{\mG}(W) = \mG(\bar{W}) + 2L\|\bar{W} - W\|^2$. 
It then follows from the update of $U^k$ in \eqref{eq:grad-descent-intro} that
\begin{align*}
& \hat{\mG}(U^k) = \min_V \mG(V) + 2L\|V - U^k\|^2 \\
& \leq \mG(\bar{W}^{k-1}) + 2L\|\bar{W}^{k-1} - U^k\|^2 \\
& = \mG(\bar{W}^{k-1}) + 2L\|\bar{W}^{k-1} - W^{k-1} + \alpha_k\nabla \mA(W^{k-1})\|^2 \\
& = \mG(\bar{W}^{k-1}) + 2L\|\bar{W}^{k-1} - W^{k-1}\|^2 + 2\alpha_k^2L\|\nabla \mA(W^{k-1})\|^2 \\
& \quad + 4\alpha_kL\langle \nabla\mA(W^{k-1}), \bar{W}^{k-1} - W^{k-1}\rangle  \\
& = \hat{\mG}(W^{k-1}) + 2\alpha_k^2L\|\nabla \mA(W^{k-1})\|^2 \\
& \quad + 4\alpha_kL\langle \nabla\mA(W^{k-1}), \bar{W}^{k-1} - W^{k-1}\rangle.
\end{align*}
By Assumption \ref{ass:bound}, we have $\|\nabla\mA(W^{k-1})\|\leq B/\lambda$. Besides, since $\nabla \mA$ is Lipschitz continuous with Lipschitz constant $L/\lambda$, it holds that
$$ 
\begin{aligned}
& \mA(\bar{W}^{k-1}) - \mA(W^{k-1}) - \langle \nabla\mA(W^{k-1}), \bar{W}^{k-1} - W^{k-1}\rangle \\
& \geq -\frac{L}{2\lambda}\|\bar{W}^{k-1} - W^{k-1}\|^2, 
\end{aligned}
$$
see, {\it e.g.}, \cite{nesterov2013introductory}. Thus, we obtain
\begin{equation}
\label{eq:decrease-D}
\begin{aligned}
\hat{\mG}(U^k) & \leq \hat{\mG}(W^{k-1}) + 4\alpha_kL\left(\mA(\bar{W}^{k-1}) - \mA(W^{k-1})\right) \\
& \quad + \frac{2\alpha_kL^2}{\lambda}\|\bar{W}^{k-1} - W^{k-1}\|^2 + \frac{2\alpha_k^2LB^2}{\lambda^2}. 
\end{aligned}
\end{equation}
Moreover, by the update of $W^k$ in \eqref{eq:ppa-intro} and the fact that $\mF$ is continuously differentiable, we know that
\begin{equation}
\label{eq:opt-F}
\nabla \mF(W^k) + \frac{\lambda}{\alpha_k}(W^k - U^k) = 0.
\end{equation} 
This, together with \eqref{eq:envelope-func}, yields
\begin{align*}
& \hat{\mG}(W^k) = \min_V \mG(V) + 2L\|V - W^k\|^2 \\
& \leq \mG(\bar{U}^k) + 2L\|\bar{U}^k - W^k\|^2 \\
& = \mG(\bar{U}^k) + 2L\left\|\bar{U}^k - U^k + \frac{\alpha_k}{\lambda}\nabla\mF(W^k) \right\|^2 \\
& = \mG(\bar{U}^k) + 2L\left\|\bar{U}^k - U^k\right\|^2 \\
& \quad + \frac{4\alpha_kL}{\lambda}\langle \nabla\mF(W^k), \bar{U}^k - U^k \rangle + \frac{2\alpha_k^2L}{\lambda^2}\|\nabla\mF(W^k)\|^2 \\
& = \hat{\mG}(U^k)+ \frac{4\alpha_kL}{\lambda}\langle \nabla\mF(W^k), \bar{U}^k - W^k \rangle \\
& \quad + \frac{4\alpha_kL}{\lambda}\langle \nabla\mF(W^k), W^k - U^k \rangle + \frac{2\alpha_k^2L}{\lambda^2}\|\nabla\mF(W^k)\|^2 \\
& \leq \hat{\mG}(U^k) + \frac{4\alpha_kL}{\lambda}\langle \nabla\mF(W^k), \bar{U}^k - W^k \rangle +  \frac{2\alpha_k^2L}{\lambda^2}\|\nabla\mF(W^k)\|^2,
\end{align*}
where the last inequality uses $\langle \nabla \mF(W^k), W^k - U^k\rangle \leq 0$, which follows from \eqref{eq:opt-F}. By Assumption~\ref{ass:bound}, we have $\|\nabla\mF(W^k)\| \leq B$. Besides, since $\nabla\mF$ is Lipschitz continuous with Lipschitz constant $L$, it holds that
$$ \mF(\bar{U}^k) - \mF(W^k) - \langle \nabla \mF(W^k), \bar{U}^k - W^k \rangle \geq -\frac{L}{2}\|\bar{U}^k - W^k\|^2. $$
Thus, we obtain
\begin{equation}
\label{eq:decrease-F}
\begin{aligned}
\hat{\mG}(W^k) & \leq \hat{\mG}(U^k) + \frac{4\alpha_kL}{\lambda}\left(\mF(\bar{U}^k) - \mF(W^k)\right) \\
& \quad + \frac{2\alpha_kL^2}{\lambda}\|\bar{U}^k - W^k\|^2 + \frac{2\alpha_k^2LB^2}{\lambda^2}. 
\end{aligned}
\end{equation}
Next, we claim
\begin{equation}
\label{eq:Lipschitz-enve}
\|\bar{W}^{k-1} - \bar{U}^k\| \leq 2\|W^{k-1} - U^k\| \leq \frac{2\alpha_kB}{\lambda}.
\end{equation}
Indeed, by \eqref{eq:envelope-func} and the definition of $\bar{W}^{k-1}$ and $\bar{U}^k$, 
we have
$$ 
\begin{aligned}
\nabla \mG(\bar{W}^{k-1}) + 4L(\bar{W}^{k-1} - W^{k-1}) & = 0, \\
\nabla \mG(\bar{U}^{k}) + 4L(\bar{U}^{k} -U^{k}) & = 0, 
\end{aligned}
$$
which implies that
\begin{equation}
\label{eq:inner-prod}
\begin{aligned}
& \langle \mG(\bar{W}^{k-1}) - \mG(\bar{U}^k), \bar{W}^{k-1} - \bar{U}^k \rangle \\
& = 4L\langle W^{k-1} - U^k, \bar{W}^{k-1} - \bar{U}^k \rangle - 4L\|\bar{W}^{k-1} - \bar{U}^k\|^2.
\end{aligned}
\end{equation} 
On the other hand, since $\nabla \mF$ and $\nabla \mA$ are Lipschitz continuous with constants $L$ and $L/\lambda$, respectively, and $\mG = \mF + \lambda\mA$, we know that $\nabla \mG$ is Lipschitz continuous with Lipschitz constant $2L$. It then follows that
\begin{align*}
& \mG(\bar{W}^{k-1}) - \mG(\bar{U}^k) - \langle \nabla \mG(\bar{U}^k), \bar{W}^{k-1} - \bar{U}^k \rangle \\
& \geq -L\|\bar{W}^{k-1} - \bar{U}^k\|^2, \\
& \mG(\bar{U}^k) - \mG(\bar{W}^{k-1}) - \langle \nabla \mG(\bar{W}^{k-1}), \bar{U}^k - \bar{W}^{k-1} \rangle \\
& \geq -L\|\bar{W}^{k-1} - \bar{U}^k\|^2,
\end{align*}
which, by adding up the two inequalities, yields
$$ \langle \mG(\bar{W}^{k-1}) - \mG(\bar{U}^k), \bar{W}^{k-1} - \bar{U}^k \rangle \geq -2L\|\bar{W}^{k-1} - \bar{U}^k\|^2. $$
By this and \eqref{eq:inner-prod}, we obtain
$$ 
\begin{aligned}
& \|\bar{W}^{k-1} - \bar{U}^k\|^2 \leq 2\langle W^{k-1} - U^k, \bar{W}^{k-1} - \bar{U}^k \rangle \\
& \leq 2\|W^{k-1} - U^k\|\|\bar{W}^{k-1} - \bar{U}^k\| 
\end{aligned}
$$
and thus the first inequality in \eqref{eq:Lipschitz-enve} holds. The second inequality in \eqref{eq:Lipschitz-enve} follows directly from \eqref{eq:grad-descent-intro} and Assumption \ref{ass:bound}. Besides, by \eqref{eq:grad-descent-intro}, \eqref{eq:ppa-intro}, and Assumption \ref{ass:bound}, we have
\begin{equation}
\label{eq:wk-wk-1}
\begin{aligned}
& \|W^k - W^{k-1}\| = \left\| U^k - \frac{\alpha_k}{\lambda}\nabla \mF(W^k) - W^{k-1}\right\| \\
& = \left\|\alpha_k\nabla \mA(W^{k-1}) + \frac{\alpha_k}{\lambda}\nabla\mF(W^k)\right\| \leq \frac{2\alpha_kB}{\lambda}.
\end{aligned}
\end{equation}
Then, by \eqref{eq:Lipschitz-enve}, \eqref{eq:wk-wk-1}, the Lipschitz continuity of $\nabla \mF$, and Assumption \ref{ass:bound}, we derive
\begin{align*}
& \mF(\bar{U}^k) - \mF(W^k) \\
& = \mF(\bar{U}^k) - \mF(\bar{W}^{k-1}) + \mF(\bar{W}^{k-1}) - \mF(W^{k-1}) \\
& \quad + \mF(W^{k-1}) - \mF(W^k) \\
& \leq  \mF(\bar{W}^{k-1}) - \mF(W^{k-1}) + B\|\bar{U}^k - \bar{W}^{k-1}\| \\
& \quad + B\|W^{k-1} - W^k\| \\
& \leq \mF(\bar{W}^{k-1}) - \mF(W^{k-1}) + \frac{4\alpha_kB^2}{\lambda},
\end{align*}

\newcommand{\figsizetwo}{0.34\textwidth}
\begin{figure*}[t]
    % \vspace{-0.05in}
    \centering
    \begin{subfigure}[b]{\figsizetwo}
        \centering
        \includegraphics[width=\textwidth]{figures/MNIST_PracticalNonIID.pdf}
        % \caption{$noise 20\%$}
        % \label{subfig:no20}
    \end{subfigure}
        \begin{subfigure}[b]{\figsizetwo}
        \centering
        \includegraphics[width=\textwidth]{figures/FMNIST_PracticalNonIID.pdf}
        % \caption{$noise 40\%$}
        % \label{subfig:no40}
    \end{subfigure}
        \begin{subfigure}[b]{\figsizetwo}
        \centering
        \includegraphics[width=\textwidth]{figures/EMNIST_PracticalNonIID.pdf}
        % \caption{$noise 60\%$}
        % \label{subfig:no60}
    \end{subfigure}
        \begin{subfigure}[b]{\figsizetwo}
        \centering
        \includegraphics[width=\textwidth]{figures/CIFAR100_PracticalNonIID.pdf}
        % \caption{$noise 60\%$}
        % \label{subfig:no60}
    \end{subfigure}
    % \vspace{-0.25in}
    
    \caption{Performance of {FedAMP} and {HeurFedAMP} compared with baselines for practical non-IID data sets.}
    % \vspace{-0.2in}
    \label{fig:original}
\end{figure*}

and
\begin{align*}
& \|\bar{U}^k - W^k\|^2 \\
& = \|\bar{U}^k - \bar{W}^{k-1} + \bar{W}^{k-1} - W^{k-1} + W^{k-1} - W^k\|^2 \\
& \leq 4\|\bar{U}^k - \bar{W}^{k-1}\|^2 + 2\|\bar{W}^{k-1} - W^{k-1}\|^2 \\
& \quad + 4\|W^{k-1} - W^k\|^2 \\
& \leq \frac{32\alpha_k^2B^2}{\lambda^2} + 2\|\bar{W}^{k-1} - W^{k-1}\|^2,
\end{align*}
where we use the inequality $(a+b+c)^2\leq 2a^2 + 4b^2 + 4c^2$ for any $a,b,c\in\R$. Combining the above two inequalities with \eqref{eq:decrease-F} gives us
\begin{equation}
\label{eq:change-in-F}
\begin{aligned}
& \hat{\mG}(W^k) \\
& \leq \hat{\mG}(U^k) + \frac{4\alpha_kL}{\lambda}\left(\mF(\bar{W}^{k-1}) - \mF(W^{k-1})\right) \\
& \quad + \frac{4\alpha_kL^2}{\lambda}\|\bar{W}^{k-1} - W^{k-1}\|^2 + \frac{18\alpha_k^2LB^2}{\lambda^2} + \frac{64\alpha_k^3L^2B^2}{\lambda^3}.
\end{aligned}
\end{equation}
Upon adding \eqref{eq:decrease-D} with \eqref{eq:change-in-F} and using $\mG = \mF + \lambda \mA$, we obtain
\begin{equation}\label{eq:total-step-1}
\begin{aligned}
& \hat{\mG}(W^k) \\
& \leq \hat{\mG}(W^{k-1}) + \frac{4\alpha_kL}{\lambda}\left(\mG(\bar{W}^{k-1}) - \mG(W^{k-1})\right) \\
& \quad + \frac{6\alpha_kL^2}{\lambda}\|\bar{W}^{k-1} - W^{k-1}\|^2 + \frac{20\alpha_k^2LB^2}{\lambda^2} + \frac{64\alpha_k^3L^2B^2}{\lambda^3} \\
& = \hat{\mG}(W^{k-1}) + \frac{4\alpha_kL}{\lambda}\left(\mG(\bar{W}^{k-1}) - \mG(W^{k-1}) \right. \\
& \quad \left. + 2L\|\bar{W}^{k-1} - W^{k-1}\|^2\right) - \frac{2\alpha_kL^2}{\lambda}\|\bar{W}^{k-1} - W^{k-1}\|^2 \\
& \quad + \frac{20\alpha_k^2LB^2}{\lambda^2} + \frac{64\alpha_k^3L^2B^2}{\lambda^3}.
\end{aligned}
\end{equation}
By the definition of $\bar{W}^{k-1}$ and \eqref{eq:envelope-func}, we know that $\mG(\bar{W}^{k-1}) + 2L\|\bar{W}^{k-1} - W^{k-1}\|^2 \leq \mG(W^{k-1})$. This, together with \eqref{eq:total-step-1}, yields
\begin{equation}
\label{eq:nonconvex-recur}
\begin{aligned}
\hat{\mG}(W^k) & \leq \hat{\mG}(W^{k-1}) - \frac{2\alpha_kL^2}{\lambda}\|\bar{W}^{k-1} - W^{k-1}\|^2 \\
& \quad + \frac{20\alpha_k^2LB^2}{\lambda^2} + \frac{64\alpha_k^3L^2B^2}{\lambda^3}.
\end{aligned} 
\end{equation}
We now consider the case where $\alpha_k = \alpha = \lambda/\sqrt{K}$ for all $k=1,2,\dots,K$. By summing up \eqref{eq:nonconvex-recur} from $k=1$ to $k=K$, we obtain
\begin{equation}
\label{eq:after-sum}
\begin{aligned}
& \min_{0\leq k\leq K} \|\bar{W}^k - W^k\|^2 \leq 
\frac{1}{K}\sum_{k=1}^K \|\bar{W}^{k-1} - W^{k-1}\|^2 \\
& \leq \frac{\lambda}{2\alpha L^2}\cdot\frac{\hat{\mG}(W^0) - \hat{\mG}(W^k)}{K} + \frac{10\alpha B^2}{\lambda L} + \frac{32\alpha^2B^2}{\lambda^2}. 
\end{aligned}
\end{equation}

\begin{figure*}[t]
    % \vspace{-0.05in}
    \centering
    \begin{subfigure}[b]{\figsizetwo}
        \centering
        \includegraphics[width=\textwidth]{figures/MNIST_RandomEpoch.pdf}
        % \caption{$noise 20\%$}
        % \label{subfig:no20}
    \end{subfigure}
        \begin{subfigure}[b]{\figsizetwo}
        \centering
        \includegraphics[width=\textwidth]{figures/FMNIST_RandomEpoch.pdf}
        % \caption{$noise 40\%$}
        % \label{subfig:no40}
    \end{subfigure}
        \begin{subfigure}[b]{\figsizetwo}
        \centering
        \includegraphics[width=\textwidth]{figures/EMNIST_RandomEpoch.pdf}
        % \caption{$noise 60\%$}
        % \label{subfig:no60}
    \end{subfigure}
        \begin{subfigure}[b]{\figsizetwo}
        \centering
        \includegraphics[width=\textwidth]{figures/CIFAR100_RandomEpoch.pdf}
        % \caption{$noise 60\%$}
        % \label{subfig:no60}
    \end{subfigure}
    % \vspace{-0.25in}
    
    \caption{Performance of {FedAMP} and {HeurFedAMP} compared with baselines for heterogeneous training.}
    % \vspace{-0.2in}
    \label{fig:randomepoch}
\end{figure*}

From \eqref{eq:envelope-func}, one can verify that
$$ \hat{\mG}(W^0) \leq \mG(W^0), \quad \mbox{and} \quad \hat{\mG}(W^k) \geq \mG^*, $$
where $\mG^*$ is the optimal value of \eqref{eq:our-form}. Also, using the definition of $\bar{W}^k$, we obtain by taking the optimality condition of \eqref{eq:envelope-func} that
$$ \nabla \mG(\bar{W}^k) + 4L(\bar{W}^k - W^k) = 0, $$
which, together with the fact that $\nabla \mG$ is Lipschitz continuous with Lipschitz constant $2L$, implies that
\begin{equation}\label{eq:G-less}
\begin{aligned}
\|\nabla \mG(W^k)\| & \leq \|\nabla \mG(\bar{W}^k)\| + \|\nabla \mG(\bar{W}^k) - \nabla\mG(W^k)\| \\
& \leq 6L\|\bar{W}^k - W^k\|. 
\end{aligned}
\end{equation}
By these, \eqref{eq:after-sum}, and $\alpha = \lambda/\sqrt{K}$, we have
$$ 
\begin{aligned}
& \min_{0\leq k\leq K}\|\nabla \mG(W^k)\|^2 \\
& \leq \frac{18(\mG(W^0) - \mG^* + 20LB^2)}{\sqrt{K}} + \mathcal{O}\left(\frac{1}{K}\right)
% = \mathcal{O}\left( \frac{\mG(W^0) - \mG^* + LB^2}{\sqrt{K}}\right) 
\end{aligned}
$$
as desired. Besides, upon summing up \eqref{eq:nonconvex-recur} from $k=1$, one has
\begin{align*}
& \sum_{k=1}^\infty\alpha_k\|\bar{W}^{k-1} - W^{k-1}\|^2 \\
& \leq \frac{\lambda}{2L^2}\hat{\mG}(W^0) + \frac{10B^2}{\lambda L}\sum_{k=1}^\infty\alpha_k^2 + \frac{32B^2}{\lambda^2}\sum_{k=1}^\infty\alpha_k^3.
\end{align*}
Then, for the case where $\alpha_k$ satisfies $\sum_{k=1}^\infty\alpha_k = \infty$ and $\sum_{k=1}^\infty\alpha_k^2 < \infty$, we obtain
$$ \sum_{k=1}^\infty\alpha_k\|\bar{W}^{k-1} - W^{k-1}\|^2 < \infty, $$
which, together with $\sum_{k=1}^\infty\alpha_k = \infty$ and $\alpha_k>0$ for all $K$, yields that
$$ \liminf_{k\rightarrow\infty}\|\bar{W}^{k-1} - W^{k-1}\| = 0. $$
The second result in Theorem \ref{thm:analysis-ncvx} then follows from this and \eqref{eq:G-less}.

\newcommand{\figsize}{0.3\textwidth}
\begin{figure*}[t]
    % \vspace{-0.05in}
    \centering
    \begin{subfigure}[b]{\figsize}
        \centering
        \includegraphics[width=\textwidth]{figures/MNIST_Drop10.pdf}
        % \caption{$noise 20\%$}
        % \label{subfig:no20}
    \end{subfigure}
        \begin{subfigure}[b]{\figsize}
        \centering
        \includegraphics[width=\textwidth]{figures/MNIST_Drop30.pdf}
        % \caption{$noise 40\%$}
        % \label{subfig:no40}
    \end{subfigure}
        \begin{subfigure}[b]{\figsize}
        \centering
        \includegraphics[width=\textwidth]{figures/MNIST_Drop50.pdf}
        % \caption{$noise 60\%$}
        % \label{subfig:no60}
    \end{subfigure}
    % \vspace{-0.25in}
    
    \caption{Performance of {FedAMP} and {HeurFedAMP} compared with baselines for different number of dropped clients on MNIST.}
    % \vspace{-0.2in}
    \label{fig:dr_MNIST}
\end{figure*}

\begin{figure*}[t]
    % \vspace{-0.05in}
    \centering
    \begin{subfigure}[b]{\figsize}
        \centering
        \includegraphics[width=\textwidth]{figures/FMNIST_Drop10.pdf}
        % \caption{$noise 20\%$}
        % \label{subfig:no20}
    \end{subfigure}
        \begin{subfigure}[b]{\figsize}
        \centering
        \includegraphics[width=\textwidth]{figures/FMNIST_Drop30.pdf}
        % \caption{$noise 40\%$}
        % \label{subfig:no40}
    \end{subfigure}
        \begin{subfigure}[b]{\figsize}
        \centering
        \includegraphics[width=\textwidth]{figures/FMNIST_Drop50.pdf}
        % \caption{$noise 60\%$}
        % \label{subfig:no60}
    \end{subfigure}
    % \vspace{-0.25in}
    
    \caption{Performance of {FedAMP} and {HeurFedAMP} compared with baselines for different number of dropped clients on FMNIST.}
    % \vspace{-0.2in}
    \label{fig:dr_FMNIST}
\end{figure*}

\begin{figure*}[t]
    % \vspace{-0.05in}
    \centering
    \begin{subfigure}[b]{\figsize}
        \centering
        \includegraphics[width=\textwidth]{figures/EMNIST_Drop10.pdf}
        % \caption{$noise 20\%$}
        % \label{subfig:no20}
    \end{subfigure}
        \begin{subfigure}[b]{\figsize}
        \centering
        \includegraphics[width=\textwidth]{figures/EMNIST_Drop30.pdf}
        % \caption{$noise 40\%$}
        % \label{subfig:no40}
    \end{subfigure}
        \begin{subfigure}[b]{\figsize}
        \centering
        \includegraphics[width=\textwidth]{figures/EMNIST_Drop50.pdf}
        % \caption{$noise 60\%$}
        % \label{subfig:no60}
    \end{subfigure}
    %     \begin{subfigure}[b]{0.14\textwidth}
    %     \includegraphics[width=\textwidth]{figures/legend3.pdf}
    %     % \label{subfig:nolegend}
    % \end{subfigure}
    % \vspace{-0.25in}
    
    \caption{Performance of {FedAMP} and {HeurFedAMP} compared with baselines for different number of dropped clients on EMNIST.}
    % \vspace{-0.2in}
    \label{fig:dr_EMNIST}
\end{figure*}

\begin{figure*}[t]
    % \vspace{-0.05in}
    \centering
    \begin{subfigure}[b]{\figsize}
        \centering
        \includegraphics[width=\textwidth]{figures/CIFAR100_Drop10.pdf}
        % \caption{$noise 20\%$}
        % \label{subfig:no20}
    \end{subfigure}
        \begin{subfigure}[b]{\figsize}
        \centering
        \includegraphics[width=\textwidth]{figures/CIFAR100_Drop30.pdf}
        % \caption{$noise 40\%$}
        % \label{subfig:no40}
    \end{subfigure}
        \begin{subfigure}[b]{\figsize}
        \centering
        \includegraphics[width=\textwidth]{figures/CIFAR100_Drop50.pdf}
        % \caption{$noise 60\%$}
        % \label{subfig:no60}
    \end{subfigure}
    % \vspace{-0.25in}
    
    \caption{Performance of {FedAMP} and {HeurFedAMP} compared with baselines for different number of dropped clients on CIFAR100.}
    % \vspace{-0.2in}
    \label{fig:dr_CIFAR100}
\end{figure*}

\section{Experiments} \label{sec:supexp}
In this section, we provide details of our experiments and more extensive experimental results to compare the empirical convergence of FedAMP and HeurFedAMP with FedAvg-FT, FedProx-FT, FedAvg, FedProx, and Separate in the practical non-IID data setting under three scenarios, i.e., regular local training, heterogeneous training, and dropped clients. All the compared methods are implemented in the same environment as described in Section~\ref{sec:exp}.

\subsection{Settings of Data Sets} \label{subsec:supexp-details}
As detailed below, we describe how we prepare the practical non-IID data settings for MNIST~\cite{lecun2010mnist}, FMNIST (Fashion-MNIST)~\cite{xiao2017fashion}, and CIFAR100~\cite{krizhevsky2009learning} data sets, which is similar to the preparation for EMNIST as described in Section~\ref{subsec:expres}.

% First, we set up 62 clients numbered as clients 0-61 and divide them into three groups.
% Then, we assign samples to the clients such that 80\% of the data of every client are uniformly sampled from a set of dominating classes, and 20\% of the data are uniformly sampled from the rest of the classes.
% Specifically, the first group consists of clients 0-9, where each client has 1000 training samples from the dominating classes with digit labels from `0' to `9'.
% The second group consists of clients 10-35, where each client has 700 training samples from the dominating classes of upper-case letters from `A' to `Z'. The third group consists of clients 36-61, where each client has 400 training samples from the dominating classes of lower-case letters from `a' to `z'.
% Every client has 100 testing samples with the same distribution as its training data.

\textbf{MNIST:} First, we set up 100 clients numbered as clients 0-99 and divide them into 5 groups where each group contains 20 clients. 
Then, we assign samples to the clients similarly as EMNIST data set described in Section~\ref{subsec:datasettings}, such that 80\% of the data of every client are uniformly sampled from a set of dominating classes, and 20\% of the data are uniformly sampled from the rest of the classes.
Specifically, the first group consists of clients 0-19, where each client has 500 training samples from the dominating classes with labels from `0' to `1'.
For the remaining 4 groups, which consists of clients 20-39, 40-59, 60-79 and 80-99, the numbers of training samples owned by a client of each group are 400, 300, 200 and 100, while they are gathered from the dominating classes of labels `2' to `3', `4' to `5', `6' to `7' and `8' to `9', respectively.
Every client has 100 testing samples with the same distribution as its training data.

\textbf{FMNIST:} 
% Similarly as MNIST, we set 100 clients and divides them into 5 groups where each group contains 20 clients as well.
% The training data distribution on each client is also the same as the distribution on the corresponding client.
For FMNIST data set, we set the same preparation as the preparation for MNIST data set except the number of training samples.
Each client in the first group has 600 training samples, while for each client in the remaining 4 groups has 500, 400, 300 and 200 training samples, respectively.
Same as EMNIST and MNIST, every client has 100 testing samples with the same distribution as its training data.

\textbf{CIFAR100:}
For CIFAR100, we first set up 100 clients numbered as 0-99 and then divide them into 20 groups where each group contains 5 clients. For each group of clients, we assign the samples to the clients such that 80\% of the data of every client are uniformly sampled from a set of dominating classes, and 20\% of the data are uniformly sampled from the rest of the classes. Since CIFAR100 originally has 100 classes which can be naturally grouped into 20 superclasses, we set classes in one superclass as dominated classes to one corresponding group. The number of training samples on client 1-20 (first 4 groups) is 500, while the number of training samples on client 21-40 (second 4 groups), 41-60 (third 4 groups), 61-80 (fourth 4 groups) and 81-100 (fifth 4 groups) is 400, 300, 200 and 100, respectively.
Like all the previous data sets, each client has 100 testing samples with the same distribution as its training data.

\subsection{Details of Implementations}
For all compared methods, we use the same CNN architecture as~\cite{mcmahan2016communication}
for the data sets of MNIST, FMNIST and EMNIST, and use ResNet18~\cite{He_2016_CVPR} for the more challenging data set of CIFAR100.
For all the methods and all the data settings, the batch size is $100$ and the number of epochs is $10$ in each round of local training. 

\nop{
For the more challenging CIFAR100 data set,
we use ResNet18~\cite{He_2016_CVPR}. 
}

Following the routine of training deep neural networks~\cite{kingma2014adam, reddi2018convergence, zhang2019adam}, we adopt the widely-used optimization algorithm ADAM~\cite{kingma2014adam} to conduct local training on each client for FedAvg, FedAvg-FT, FedProx, FedProx-FT, {FedAMP} and {HeurFedAMP}.
However, since both SCAFFOLD and APFL achieve personalized federated learning by their own customized optimization methods that are not compatible with ADAM, we use their own customized optimization methods by default to train their models.

\nop{
For SCAFFOLD and APFL, we use their default gradient update methods for model training, because both of them conduct personalized federated learning by deeply customized gradient update methods that are not compatible with ADAM. 
}

\nop{
We employ ADAM~\cite{kingma2014adam} as the local training optimization algorithm on each client for FedAvg/FedAvg-FT, FedProx/FedProx-FT, {FedAMP} and {HeurFedAMP}. 

It is well known that ADAM is a variant of stochastic gradient decent (SGD) optimizer for training deep neural networks which has demonstrated its superior performance over the vanilla SGD in various training tasks, \cite{kingma2014adam, reddi2018convergence, zhang2019adam}.

However, both SCAFFOLD and APFL have designed their own special updates for their local training, respectively. Thus, ADAM can not be employed by either of them. 
}

\nop{
\noindent\textbf{Hyperparameters.} 
}

For FedAvg, FedAvg-FT, FedProx, FedProx-FT, {FedAMP} and {HeurFedAMP},
we use a learning rate of $10^{-3}$ and 
iterate for $90$ communication rounds such that they all converge empirically.
For SCAFFOLD and APFL, since their customized optimization methods are different from ADAM, we tried many different learning rates, such as $10^{-6}, 10^{-5}, 10^{-4}, 10^{-3}, 10^{-2}$ and $10^{-1}$, and find the best learning rate $10^{-2}$ for both of them.
Then, we iterate for $600$ communication rounds for them to converge empirically.

As shown above, the local optimization algorithms of SCAFFOLD and APFL are different from other methods and these two methods require much more communication rounds to converge empirically. Thus, we do not include their empirical convergence results in the experiments for demonstrating the convergence of FedAMP and HeurFedAMP.
\nop{
tried many different learning rate and total communications rounds, and finally select the best learning rate as $10^{-2}$ 

after carefully tuning the learning rate and the total communication rounds, we set the learning rate as $10^{-2}$ and the total number of communication rounds as $600$ to make sure they empirically converge.
}
% \footnote{We have made large efforts to tune these hyperparameters for SCAFFOLD and APFL. However, we still find that both SCAFFOLD and APFL can occasionally stuck in a very bad local solution as shown in the experimental results, i.e., Table \ref{tab:result_NonIIDNonGrouping} and \ref{tab:result}., especially when the network becomes deeper and the distribution is more complicate.} 

\nop{
Now, we illustrate the hyperparameters of all compared methods as follows. 
}

\subsection{Settings of Hyperparameters}
For Fedprox and Fedprox-FT, we tried different regularization parameters, such as $\{10^{-i}|i \in \{0,1,2,3\}\}$, and find that $i=2$  provided best performance for all the dataset and data settings. 
For SCAFFOLD, we set its global step-size $\eta_g$ to be 1 as suggested in \cite{karimireddy2019scaffold}. 
For APFL, we tune the mixture weights $\alpha_i$ from $\{0, 0.25, 0.5, 0.75\}$ as used in \cite{deng2020adaptive} to achieve its best performance on each data set and data settings.
For {FedAMP} and {HeurFedAMP}, we set $\lambda=1$ and $\xi_{ii} = 1/(N_i +1)$  where $N_i$ is the number of same distribution clients for client $i$. In addition, we initialize $\alpha_k$ with $10^4$ and reduce it by a factor $0.1$ for every $30$ communication rounds. In addition, for FedAMP, we tune $\sigma$ from $\{10^i | i \in \{0,1,2,3,4,5,6\}\}$, while for HeurFedAMP we tune $\sigma$ from $\{1, 10, 25, 50, 75, 100\}$.
The detailed choices of tuned hyperparameters are listed in Table ~\ref{tab:hyper-IID} to~\ref{tab:hyper-non}.

\nop{
including experimental results demonstrating speed and robustness of the proposed methods.
}

\nop{
performance of {FedAMP}, {HeurFedAMP} and baselines in terms of the best mean testing accuracy for the IID data setting. 
}

\nop{
As reported in \cite{deng2020adaptive}, when $\alpha_i=0$, APFL is equivalent to FedAvg and achieves best performance for the IID data setting. Thus, we do not include the results of APFL in this setting. }
\begin{table}[h!]
\setlength{\tabcolsep}{2pt}
\caption{Values of Hyperparameters(IID)}
\label{tab:hyper-IID}
\centering
%\begin{tabular}{l|l{2cm}l{2cm}l{2cm}l{2cm}l{2cm}} 
\begin{tabular}{l|cccc} 
 \toprule
Parameter & MNIST & FMNIST & EMNIST & CIFAR100 \\ 
 \hline
%  Centralized & 99.11	& 90.03 &	73.88 &	61.83
% \\
$\sigma$({FedAMP}) & 100 & 100 & 10 & $10^6$	 \\
$\sigma$({HeurFedAMP}) & 25 & 50 & 50 &	 10\\
$\alpha_i$(APFL) & 0 & 0 & 0 & 0 \\
%$\tau$ ({FedAMP} and {HeurFedAMP}) & 0.99 & 0.99 &	0.084 & 0.99\\
 \bottomrule
\end{tabular}
\end{table}

\begin{table}[h!]
\setlength{\tabcolsep}{2pt}
\caption{Values of Hyperparameters(Pathological non-IID)}
\label{tab:hyper-path}
\centering
%\begin{tabular}{l|l{2cm}l{2cm}l{2cm}l{2cm}l{2cm}} 
\begin{tabular}{l|cccc} 
 \toprule
Parameter & MNIST & FMNIST & EMNIST & CIFAR100 \\ 
 \hline
%  Centralized & 99.11	& 90.03 &	73.88 &	61.83
% \\
$\sigma$({FedAMP}) & 100 & 10 & 10 & $10^6$	 \\
$\sigma$({HeurFedAMP}) & 25 & 100 & 50 & 10 \\
$\alpha_i$(APFL) & 0.25 & 0.25 & 0.25 & 0.25\\
%$\tau$({FedAMP} and {HeurFedAMP}) & 0.5 & 0.5 &	0.5	& 0.5\\
 \bottomrule
\end{tabular}
\end{table}

\begin{table}[h!]
\setlength{\tabcolsep}{2pt}
\caption{Values of Hyperparameters(Practical non-IID)}
\label{tab:hyper-non}
\centering
%\begin{tabular}{l|l{2cm}l{2cm}l{2cm}l{2cm}l{2cm}} 
\begin{tabular}{l|cccc} 
 \toprule
Parameter & MNIST & FMNIST & EMNIST & CIFAR100 \\ 
 \hline
%  Centralized & 99.11	& 90.03 &	73.88 &	61.83
% \\
$\sigma$({FedAMP}) & 100 & 10 & 10 & $10^6$	 \\
$\sigma$({HeurFedAMP}) & 25 & 100 & 50 & 10	 \\
$\alpha_i$(APFL) & 0.25 & 0.75 & 0.25 & 0.25\\
%$\tau $({FedAMP} and {HeurFedAMP}) & 0.95 & 0.95 & 0.9	& 0.8\\
 \bottomrule
\end{tabular}
\end{table}
% The \textit{practical} hyperparameter settings are specified as follows which achieve the optimal validation accuracy by cross validation.
\nop{\noindent\textbf{Hyperparameters.} In Section \ref{sec:exp}, we provide the common hyperparameters used for all the methods in all the experiments. Here, we provide hyperparameters chosen for {FedAMP} and {HeurFedAMP}. Second, from Table \ref{tab:hyper-IID} to \ref{tab:hyper-non}, we list all other hyperparameters which we obtain through the cross validation for each data setting. We also observe that the parameter $\sigma$'s range for {FedAMP} is very large due to the large variation of the Euclidean distance between parameters of two models in high dimension space. This is one of our motivations of proposing {HeurFedAMP} in Section~\ref{sec:instances}.
}

% \subsection{Tolerance to Dirty Data} \label{subsec:supexp-dirty}
% Besides the dirty data experiments on EMNIST data set which is shown in Section\ref{subsec:dirtydata}, we also conduct more experiments on MNIST, FMNIST and CIFAR100 to examine the tolerance of dirty data for {FedAMP}, {HeurFedAMP}, and baselines. The dirty data setting is the same as stated in Section~\ref{subsec:dirtydata}.

% The results on MNIST, FMNIST and CIFAR100 are shown in Fig.~\ref{fig:no_MNIST},~\ref{fig:no_FMNIST} and~\ref{fig:no_CIFAR}, respectively. Similar to the performance on EMNIST which is shown in Section~\ref{subsec:dirtydata}, {FedAMP} and {HeurFedAMP} all achieve the best mean validation accuracy in all three levels of dirty labels. This further confirms the effectiveness of applying the attentive message passing mechanism when encountering dirty data.
% % On CIFAR100, see Fig.~\ref{fig:no_CIFAR}, {FedAMP} and {HeurFedAMP} starts with the lower mean validation accuracy than FedAvg-FT and FedProx-FT before communication round 30. However, after round 30, {FedAMP} and {HeurFedAMP} can increasingly achieve better accuracy than FedAvg-FT and FedProx-FT.

\subsection{The Empirical Convergence Results on Non-IID Data Settings}
Fig.~\ref{fig:original} shows the empirical convergence results of FedAMP and HeurFedAMP alongside with other baselines, FedAvg, FedAvg-FT, FedProx and FedProx-FT on the practical non-IID data settings. 
Specifically, we focus on the changes of mean testing accuracy of these algorithms in each communication round.
Contributed by the attentive message passing mechanism, both FedAMP and HeurFedAMP converge to higher mean testing accuracies on all four data sets than baselines. This phenomenon does not only validate the effectiveness of the attentive message passing mechanism in collaborating the clients under the non-IID data setting, but also presents the efficiency of the training process of FedAMP and HeurFedAMP.

\subsection{Tolerance to Heterogeneous Training}
Because of the heterogeneity of the federated learning system, clients may endure different local training epochs for different time. One possible effect of this scenario is that there could be some bad local models resulted by the local training with small number of epochs.
To simulate the heterogeneous training, we train each client by a random number of epochs with expectation equal to 10 during each communication round. Specifically, this random number is uniformly drawn from an integer between [1, 19]. To analyze impacts of heterogeneous training, we plot the mean accuracy versus the communication round for all the methods in Fig.~\ref{fig:randomepoch}. We observe that FedAMP and HeurFedAMP both have high tolerance to heterogeneous training and converge to overall higher mean test accuracies on all four data sets than baselines. This confirms that by taking the advantage of attentive message passing mechanism, FedAMP and HeurFedAMP can selectively exclude bad local models out of the collaboration.

\subsection{Tolerance to Dropped Clients}\label{subsec:supexp-drop}
To address the unreliable operating environment challenge in personalized federated learning, we conduct the dropped clients experiments for FedAMP, HeurFedAMP and other baselines. 
The results of 10\%, 30\%, and 50\% randomly dropped clients in each round for the four practical non-IID data sets are shown in Fig.~\ref{fig:dr_EMNIST} to~\ref{fig:dr_CIFAR100}. We first observe that in general FedAMP and HeurFedAMP can converge to higher mean testing accuracy than baselines
for EMNIST, MNIST and FMNIST. 
For CIFAR100, {FedAMP} and {HeurFedAMP} can also converge to comparable mean testing accuracies when comparing with FedAvg-FT and FedProx-FT.
These results demonstrate that both FedAMP and HeurFedAMP can robustly handle clients dropping.
Benefiting from attentive message passing mechanism, FedAMP and HeurFedAMP are not influenced by the dropped clients as they can adpatively facilitate the pair-wise collaborations among online clients.
